# Supplementary material for: Versatile Skill Control via Self-supervised Adversarial Imitation of Unlabeled Mixed Motions
Source: arXiv:2209.07899 source file (2023-02-11)
Supplement: Supplementary file 1 [file suppl.tex]

\section{Training Details}\label{app:sec:training_details}

\subsection{Training Parameters}

    The learning networks and algorithm are implemented in PyTorch 1.10 with CUDA 11.3. Adam is used as the optimizer for the policy and value function with an adaptive learning rate with a KL divergence target of $0.01$. The discount factor $\gamma$ is set to $0.99$, the clip range $\epsilon$ is set to $0.2$, and the entropy coefficient $\alpha$ is set to $0.01$. The policy runs at $50$\,Hz. All training is done by collecting experiences from $4096$ uncorrelated instances of the simulator in parallel. Most of the experiments are executed on the cluster of Max Planck Institute for Intelligent Systems with NVIDIA A100 and Tesla V100 GPUs. In this setting, one run with $2000$ iterations with the specified compute settings and devices completes within $1$ hour. The police training information is summarized in \tabref{table:policy_training_params} and the discriminator training information is summarized in \tabref{table:discriminator_training_params}
    \begin{table}[h]
    \centering
        \caption{Policy Training parameters}
        \begin{tabular}{lcc}
        \toprule
            Parameter & Symbol & Value \\
            \midrule
            step time seconds & $-$ & $0.02$ \\
            max episode time seconds & $-$ & $20$ \\
            max iterations & $-$ & $2000$ \\
            steps per iteration & $-$ & $24$ \\
            policy learning rate & $lr^\pi$ & $0.001$ \\
            policy learning epochs & $-$ & $5$ \\
            policy mini-batches & $-$ & $4$ \\
            KL divergence target & $-$ & $0.01$ \\
            discount factor & $\gamma$ & $0.99$ \\
            clip range & $\epsilon$ & $0.2$ \\
            entropy coefficient & $\alpha$ & $0.01$ \\
            parallel training environments & $-$ & $4096$ \\
            number of seeds & $-$ & $5$ \\
            approximate training hours & $-$ & $1$ \\
        \bottomrule
        \end{tabular}
        \label{table:policy_training_params}
    \end{table}

    \begin{table}[h]
    \centering
        \caption{Discriminator Training parameters}
        \begin{tabular}{lcccc}
        \toprule
            Parameter & Symbol & \id & \sd & \oc \\
            \midrule
            ensemble size & $N$ & $1$ & $5$ & $5$ \\
            optimizer & $-$ & SGD & Adam & Adam \\
            learning rate & $lr$ & $0.0001$ & $0.0001$ & $0.00001$ \\
            weight decay & $wd$ & $0.0001$ & $0.0005$ & $0.0005$\\
            momentum & $-$ & $0.5$ & $-$ & $-$ \\
            gradient penalty weight & $\wGP$ & $5.0$ & $-$ & $-$ \\
            learning epochs & $-$ & $1$ & $1$ & $-$ \\
            mini-batches & $-$ & $80$ & $80$ & $80$ \\
            observation horizon & $H$ & $2$ & $8$ & $8$ \\
            class number & $-$ & $-$ & $N_z$ & $N_c$ \\
        \bottomrule
        \end{tabular}
        \label{table:discriminator_training_params}
    \end{table}

\subsection{Network Architecture}

The network architecture is detailed in \tabref{table:network_architecture}, where $\HI, \HS, \HC$ denote the discriminator observation horizons.

\begin{table}
    \centering
    \caption{Network architecture}
    \begin{tabular}{lcccc}
    \toprule
        Network & Symbol & Type & Shape & Activation \\
        \midrule
        policy & $\pi$ & MLP & $34+N_z, 128, 128, 128, 8$ & ELU \\
        value function & $V$ & MLP & $34+N_z, 128, 128, 128, 1$ & ELU \\
        \id & $\idisc$ & MLP & $26 \HI, 512, 256, 1$ & ReLU \\
        \sd & $\sdisc$ & MLP Ensemble & $26 \HS, 256, 256, N_z$ & ReLU \\
        \oc & $C$ & MLP Ensemble & $26 \HC, 1024, 512, N_c$ & ReLU \\
    \bottomrule
    \end{tabular}
    \label{table:network_architecture}
\end{table}

\subsection{Domain Randomization}

Two types of domain randomization techniques are applied during training to improve policy performance when transferring from simulation to the real system.

On the one hand, the base mass of the parallel training instances is perturbed with an additional weight $m' \sim \mathcal{U}(-0.5, 1.0)$, where $\mathcal{U}$ denotes uniform distribution. On the other hand, random pushing is also applied every $15$ seconds on the robot base by forcing its horizontal linear velocity to be set randomly within $v_{xy} \sim \mathcal{U}(-0.5, 0.5)$.

\section{Model Representation} \label{app:sec:model_representation}

% \subsection{Imitation Discriminator Observation} \label{app:sec:imitation_discriminator_observation}

% \tabref{table:imitation_discriminator_observation_space} lists the extracted features sent to the \id.

% \begin{table}
%     \centering
%     \caption{Imitation discriminator observation space}
%     \begin{tabular}{lcc}
%     \toprule
%         Entry & Symbol & Dimensions \\
%         \midrule
%         base linear velocity & $v$ & 0:3 \\
%         base angular velocity & $\omega$ & 3:6 \\
%         projected gravity & $g$ & 6:9 \\
%         base height & $h$ & 9:10 \\
%         joint position & $q$ & 10:18 \\
%         joint velocity & $\dot{q}$ & 18:26 \\
%     \bottomrule
%     \end{tabular}
%     \label{table:imitation_discriminator_observation_space}
% \end{table}

% The resulting features are then flattened and normalized before being used as inputs to the \id networks.

% \subsection{Skill Discriminator Observation} \label{app:sec:skill_discriminator_observation}

% \tabref{table:skill_discriminator_observation_space} lists the extracted features sent to the \sd and \oc.

% \begin{table}
%     \centering
%     \caption{Skill discriminator observation space}
%     \begin{tabular}{lcc}
%     \toprule
%         Entry & Symbol & Dimensions \\
%         \midrule
%         base linear velocity & $v$ & 0:3 \\
%         base angular velocity & $\omega$ & 3:6 \\
%     \bottomrule
%     \end{tabular}
%     \label{table:skill_discriminator_observation_space}
% \end{table}

% The resulting features are then flattened and batch-normalized before being used as inputs to the \sd and \oc networks.

\subsection{Discriminator Observation} \label{app:sec:discriminator_observation}

In our work, the \id, the \sd and the \oc share the same observation space with different horizons as detailed in \tabref{table:discriminator_training_params}. \tabref{table:discriminator_observation_space} lists the extracted features sent to the discriminators.

\begin{table}
    \centering
    \caption{Discriminator observation space}
    \begin{tabular}{lcc}
    \toprule
        Entry & Symbol & Dimensions \\
        \midrule
        base linear velocity & $v$ & 0:3 \\
        base angular velocity & $\omega$ & 3:6 \\
        projected gravity & $g$ & 6:9 \\
        base height & $h$ & 9:10 \\
        joint position & $q$ & 10:18 \\
        joint velocity & $\dot{q}$ & 18:26 \\
    \bottomrule
    \end{tabular}
    \label{table:discriminator_observation_space}
\end{table}

The resulting features are then flattened and normalized before being used as inputs to the discriminator networks.

\subsection{Policy Observation and Action Space} \label{app:sec:policy_observation}
    The policy observation space consists of 34 dimensions and one-hot encoded latent skill variable of dimension $N_z$ as detailed in \tabref{table:policy_observation_space}.

    \begin{table}
        \centering
        \caption{Policy observation space}
        \begin{tabular}{lccc}
        \toprule
            Entry & Symbol & Dimensions & noise level $b$ \\
            \midrule
            base linear velocity & $v$ & 0:3 & $0.2$ \\
            base angular velocity & $\omega$ & 3:6 & $0.05$ \\
            projected gravity & $g$ & 6:9 & $0.05$ \\
            velocity command & $c$ & 9:10 & $0.0$ \\
            joint positions & $q$ & 10:18 & $0.01$ \\
            joint velocities & $\dot{q}$ & 18:26 & $0.75$ \\
            last actions & $a'$ & 26:34 & $0.0$ \\
            latent skill & $z$ & 34:34+$N_z$ & $0.0$ \\
        \bottomrule
        \end{tabular}
        \label{table:policy_observation_space}
    \end{table}

    The noise level $b$ denotes the artificial noise added during training to increase the policy robustness.

    The action space is of 8 dimensions and encodes the target joint position for each of the 8 actuators. The PD gains are set to $5.0$ and $0.1$, respectively.

\section{Regularization Reward Functions} \label{app:sec:regularization_reward_functions}

    The regularization reward function formulations are detailed below. The set of involved hyperparameters are summarized in \tabref{table:regularization_reward_hyperparameters}.

    \begin{table}
    \centering
        \caption{Regularization reward hyperparameters}
        \begin{tabular}{lccccccc}
        \toprule
            Hyperparameter & $w_{ar}$ & $w_{q_a}$ & $w_{q_T}$ & $w_{t_f}$ & $w_{\dot{\phi}}$ & $w_{\dot{\psi}}$ & $w_{\dot{y}}$ \\
            \midrule
            Value & $-0.01$ & $-2.5 \times 10^{-7}$ & $-2.5 \times 10^{-5}$ & $1.0$ & $-0.02$ & $-0.02$ & $-0.02$ \\
            \bottomrule
        \end{tabular}
        \label{table:regularization_reward_hyperparameters}
    \end{table}

\subsection{Action Rate}

    \begin{equation}
        r_{ar} = w_{ar} \| a' - a \|_2^2,
    \end{equation}

    where $w_{ar}$ denotes the weight of the action rate reward, $a'$ and $a$ denote the previous and current actions.

\subsection{Joint Acceleration}

    \begin{equation}
        r_{q_a} = w_{q_a} \left \| \dfrac{\dot{q}' - \dot{q}}{\Delta t} \right \|_2^2,
    \end{equation}

    where $w_{q_a}$ denotes the weight of the joint acceleration reward, $\dot{q}'$ and $\dot{q}$ denote the previous and current joint velocity, $\Delta t$ denotes the step time interval.

\subsection{Joint Torque}

    \begin{equation}
        r_{q_T} = w_{q_T} \left \| T \right \|_2^2,
    \end{equation}

    where $w_{q_T}$ denotes the weight of the joint torque reward, $T$ denotes the joint torques.

\subsection{Feet Air Time}

    \begin{equation}
        r_{t_f} = w_{t_f} \sum_{i=1}^4 t_{f_i} \llbracket f_i\in \gC \rrbracket,
    \end{equation}

    where $w_{t_f}$ denotes the weight of the feet air time reward, $t_{f_i}$ denotes the time foot $i$ accumulates in the air before landing. $\gC$ is the set of foot states touching the ground, and $\llbracket \cdot \rrbracket$ is the Iverson bracket ($1$ if true, $0$ otherwise).

\subsection{Angular Velocity $x$}

    \begin{equation}
        r_{\dot{\phi}} = w_{\dot{\phi}} \left \| \dot{\phi} \right \|_2^2,
    \end{equation}

    where $w_{\dot{\phi}}$ denotes the weight of the angular velocity $x$ reward, $\dot{\phi}$ denotes the base roll rate.

\subsection{Angular Velocity $z$}

    \begin{equation}
        r_{\dot{\psi}} = w_{\dot{\psi}} \left \| \dot{\psi} \right \|_2^2,
    \end{equation}

    where $w_{\dot{\psi}}$ denotes the weight of the angular velocity $z$ reward, $\dot{\psi}$ denotes the base yaw rate.

\subsection{Linear Velocity $y$}

    \begin{equation}
        r_{\dot{y}} = w_{\dot{y}} \left \| \dot{y} \right \|_2^2,
    \end{equation}

    where $w_{\dot{y}}$ denotes the weight of the linear velocity $y$ reward, $\dot{y}$ denotes the base lateral velocity.

\section{Motions}\label{app:sec:motions}

We provide example sequences of the component motions in the diverse dataset that we learn in this work in \figref{fig:motions}.

\begin{figure}
    \centering
    \begin{subfigure}[b]{1.0\linewidth}
    \centering
        \includegraphics[width=1.0\linewidth]{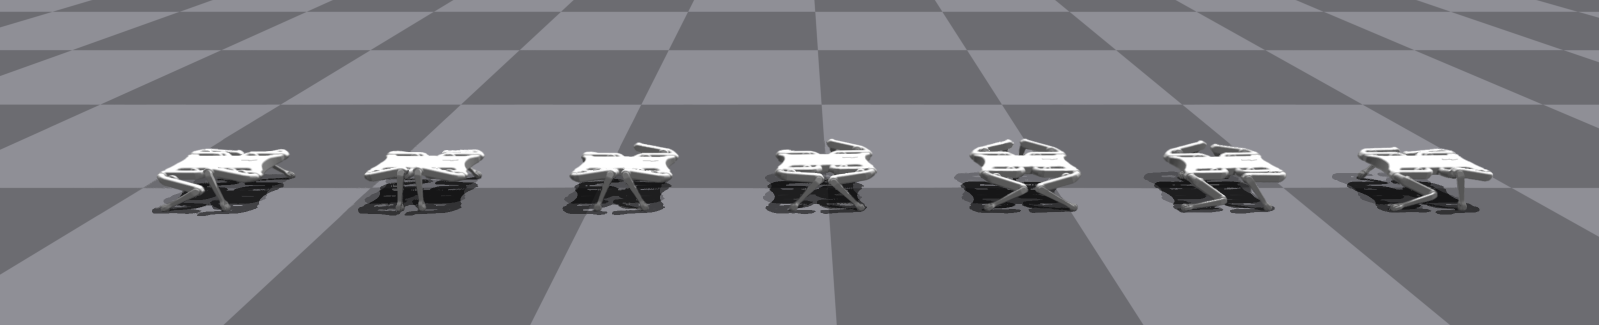}
        \caption{Crawl}
    \end{subfigure}\hspace{0.1em}
    \begin{subfigure}[b]{1.0\linewidth}
    \centering
        \includegraphics[width=1.0\linewidth]{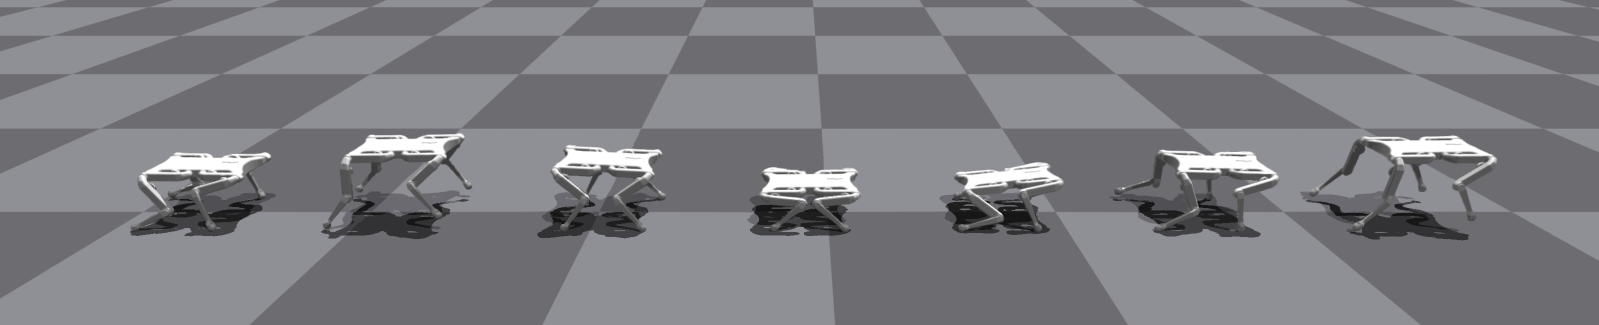}
        \caption{Leap}
    \end{subfigure}\hspace{0.1em}
    \begin{subfigure}[b]{1.0\linewidth}
    \centering
        \includegraphics[width=1.0\linewidth]{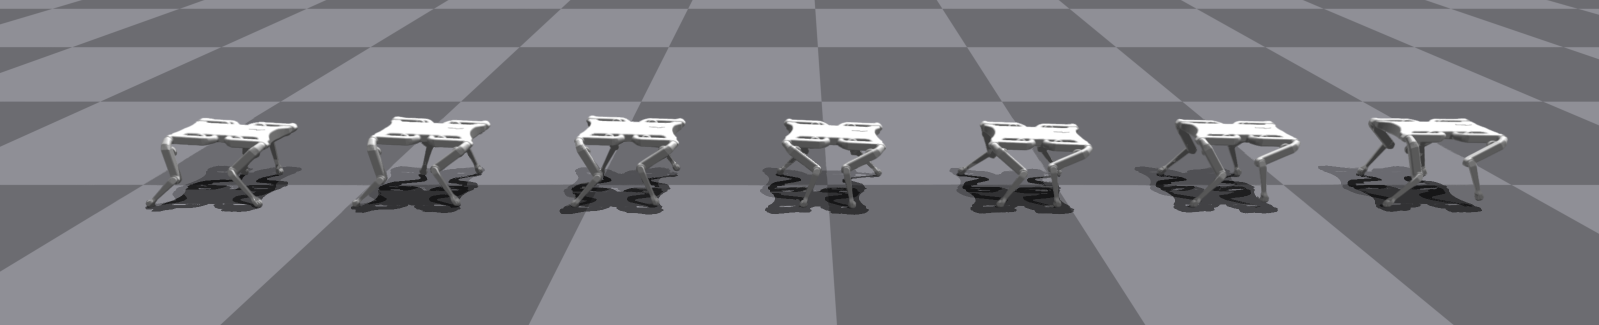}
        \caption{Stilt}
    \end{subfigure}\hspace{0.1em}
    \begin{subfigure}[b]{1.0\linewidth}
    \centering
        \includegraphics[width=1.0\linewidth]{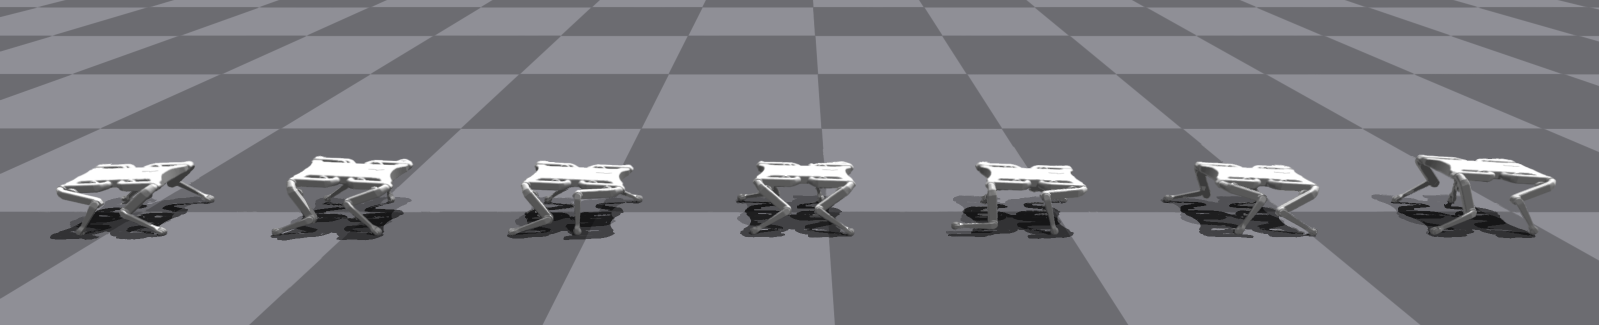}
        \caption{Trot}
    \end{subfigure}\hspace{0.1em}
    \begin{subfigure}[b]{1.0\linewidth}
    \centering
        \includegraphics[width=1.0\linewidth]{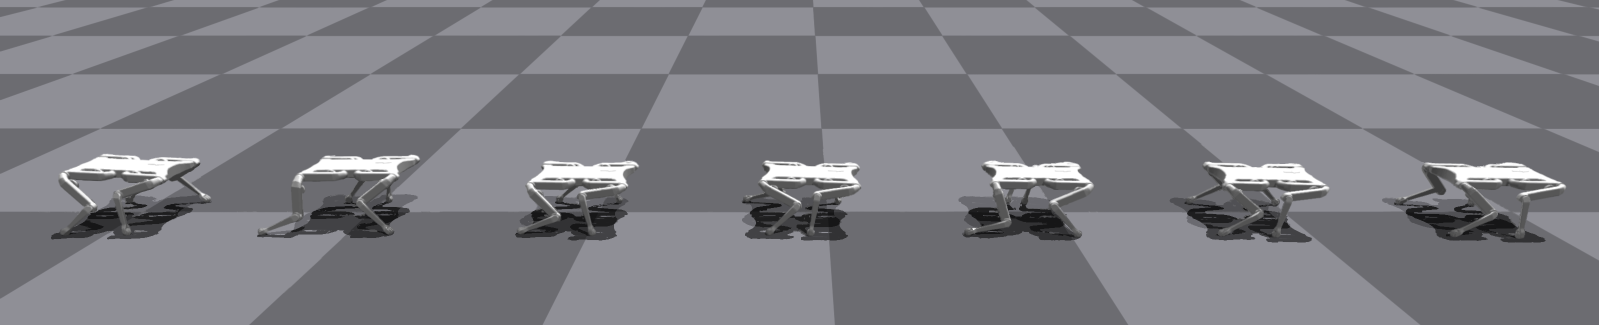}
        \caption{Walk}
    \end{subfigure}\hspace{0.1em}
    \begin{subfigure}[b]{1.0\linewidth}
    \centering
        \includegraphics[width=1.0\linewidth]{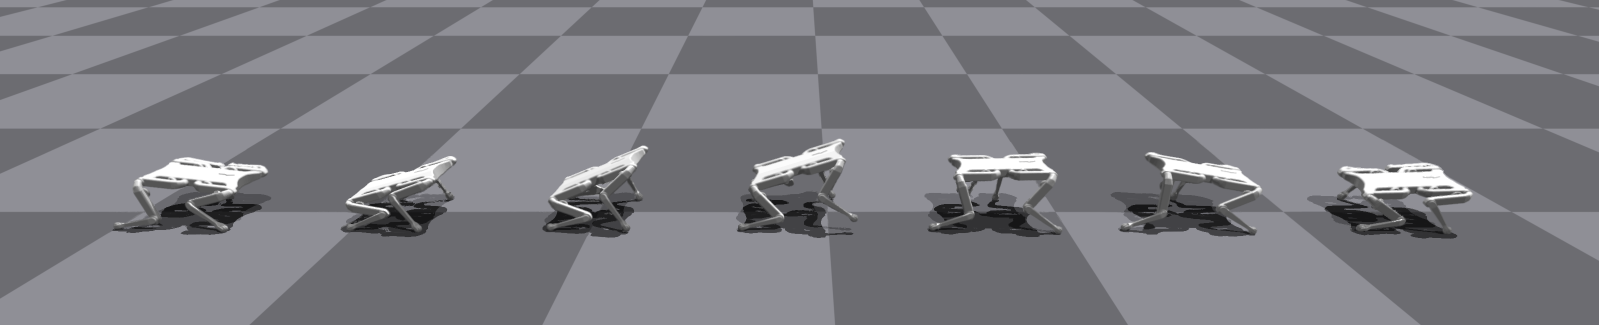}
        \caption{Wave}
    \end{subfigure}\hspace{0.1em}
    \caption{Example sequences of component motions in the diverse dataset in simulation.}
    \label{fig:motions}
\end{figure}
